# Supplementary material for: Beyond Backprop: Online Alternating Minimization with Auxiliary Variables
Source: arXiv:1806.09077 source file (2019-06-05)
Supplement: Supplementary file 1 [file supplement.tex]

\relax
%File: formatting-instruction.tex
\documentclass[letterpaper]{article} %DO NOT CHANGE THIS
\usepackage{aaai19}  %Required
\usepackage{times}  %Required
\usepackage{helvet}  %Required
\usepackage{courier}  %Required
\usepackage{url}  %Required
\usepackage{graphicx}  %Required
\frenchspacing  %Required

\usepackage[utf8]{inputenc} % allow utf-8 input
\usepackage[T1]{fontenc}    % use 8-bit T1 fonts
\usepackage{hyperref}       % hyperlinks
\usepackage{url}            % simple URL typesetting
\usepackage{booktabs}       % professional-quality tables
\usepackage{amsfonts}       % blackboard math symbols
\usepackage{nicefrac}       % compact symbols for 1/2, etc.
\usepackage{microtype}      % microtypography

%%%%%% added by IR
% use Times
\usepackage{times}
% For figureshttps://www.overleaf.com/12788364nyrdrrtcdrht#
\usepackage{graphicx} % more modern
\usepackage{subfigure}
% Recommended, but optional, packages for figures and better typesetting:
\usepackage{microtype}
\usepackage{booktabs} % for professional tables

% For citations
%\usepackage{natbib}

% For algorithms
\usepackage{algorithm}
\usepackage{algorithmic}
%\usepackage{algorithmicx}

% As of 2011, we use the hyperref package to produce hyperlinks in the
% resulting PDF.  If this breaks your system, please commend out the
% following usepackage line and replace \usepackage{icml2016} with
% \usepackage[nohyperref]{icml2016} above.
\usepackage{hyperref}

\usepackage{url}
\usepackage{tikz}
\usepackage{fancyhdr} 
\usepackage{color}
\usepackage{epsf}
\usepackage{epsfig}
\usepackage{bm}
\usepackage{bbm}
\usepackage{amsmath, amssymb}
\usepackage{amsfonts}
\usepackage{mathtools}
\usepackage{amsthm}
\usepackage{comment}
\usepackage{caption}
\usepackage{multirow}
% added by RL
\usepackage{setspace}
\usepackage{xr}

% added by IR
\usepackage{verbatim}
\usepackage{booktabs}
\usepackage{epstopdf}
\usepackage{lipsum}
\usepackage{url}

\usepackage{multicol}
%

% hyperref makes hyperlinks in the resulting PDF.
% If your build breaks (sometimes temporarily if a hyperlink spans a page)
% please comment out the following usepackage line and replace
% \usepackage{icml2018} with \usepackage[nohyperref]{icml2018} above.
\usepackage{hyperref}

% Attempt to make hyperref and algorithmic work together better:
%\newcommand{\theHalgorithm}{\arabic{algorithm}}

% \DeclareMathOperator{\MIF}{MI} 

%\newtheorem{lemma}{Lemma}
%\newtheorem{theorem}[lemma]{Theorem}
%\newtheorem{corollary}[lemma]{Corollary}

%

%additions suggested by Sahil

%deletions suggested by Sahil

\newcommand{\shrink}[1]{}

\definecolor{shadecolor}{gray}{0.95}

\newlength\myindent
\setlength\myindent{2em}

\setlength{\pdfpagewidth}{8.5in}  %Required
\setlength{\pdfpageheight}{11in}  %Required

\setcounter{secnumdepth}{2}

 \begin{document}
% The file aaai.sty is the style file for AAAI Press 
% proceedings, working notes, and technical reports.
%

%\title{Beyond Backpropagation: \\ Alternating Minimization with co-Activation Memory}

%\title{Beyond Backprop: Breaking Gradient Chains with \\ Auxiliary   Variables in Online  Alternating Minimization   }

\externaldocument{AltMin_AAAI2019}
\appendix
\onecolumn

\centerline{\bf \Large Supplemental Material}
\section{Proofs}
\input{./sec_supplement.tex}

\end{document}
